# Supplementary material for: Magnifying What Matters: Attention-Guided Adaptive Rendering for Visual Text Comprehension
Source: arXiv:2606.12898 source file (2026-06-11)
Supplement: Supplementary file 1 [file appendix_back_up.tex]

% !TEX root = ../neurips_2026.tex
\section{Full $(k,\alpha)$ Sensitivity Sweep}
\label{app:sensitivity}

Fig.~\ref{fig:sensitivity_full} extends the headline 1$\times$2 view of
\S\ref{sec:exp:analysis} (HotpotQA + LB-QP) to all 12 datasets used in
\S\ref{sec:exp:main}. Each panel reports enhanced F1 (\%) at every
$(k,\alpha) \in \{0.5\%, 1\%, 2\%, 5\%, 10\%\} \times \{1.2, 1.5, 1.8, 2.0\}$
cell; the translucent grey plane (red dashed wireframe) marks the
Plain~VQA baseline, and per-panel colour is normalised to the panel's
own range.

\begin{figure}[h]
  \centering
  \includegraphics[width=\linewidth]{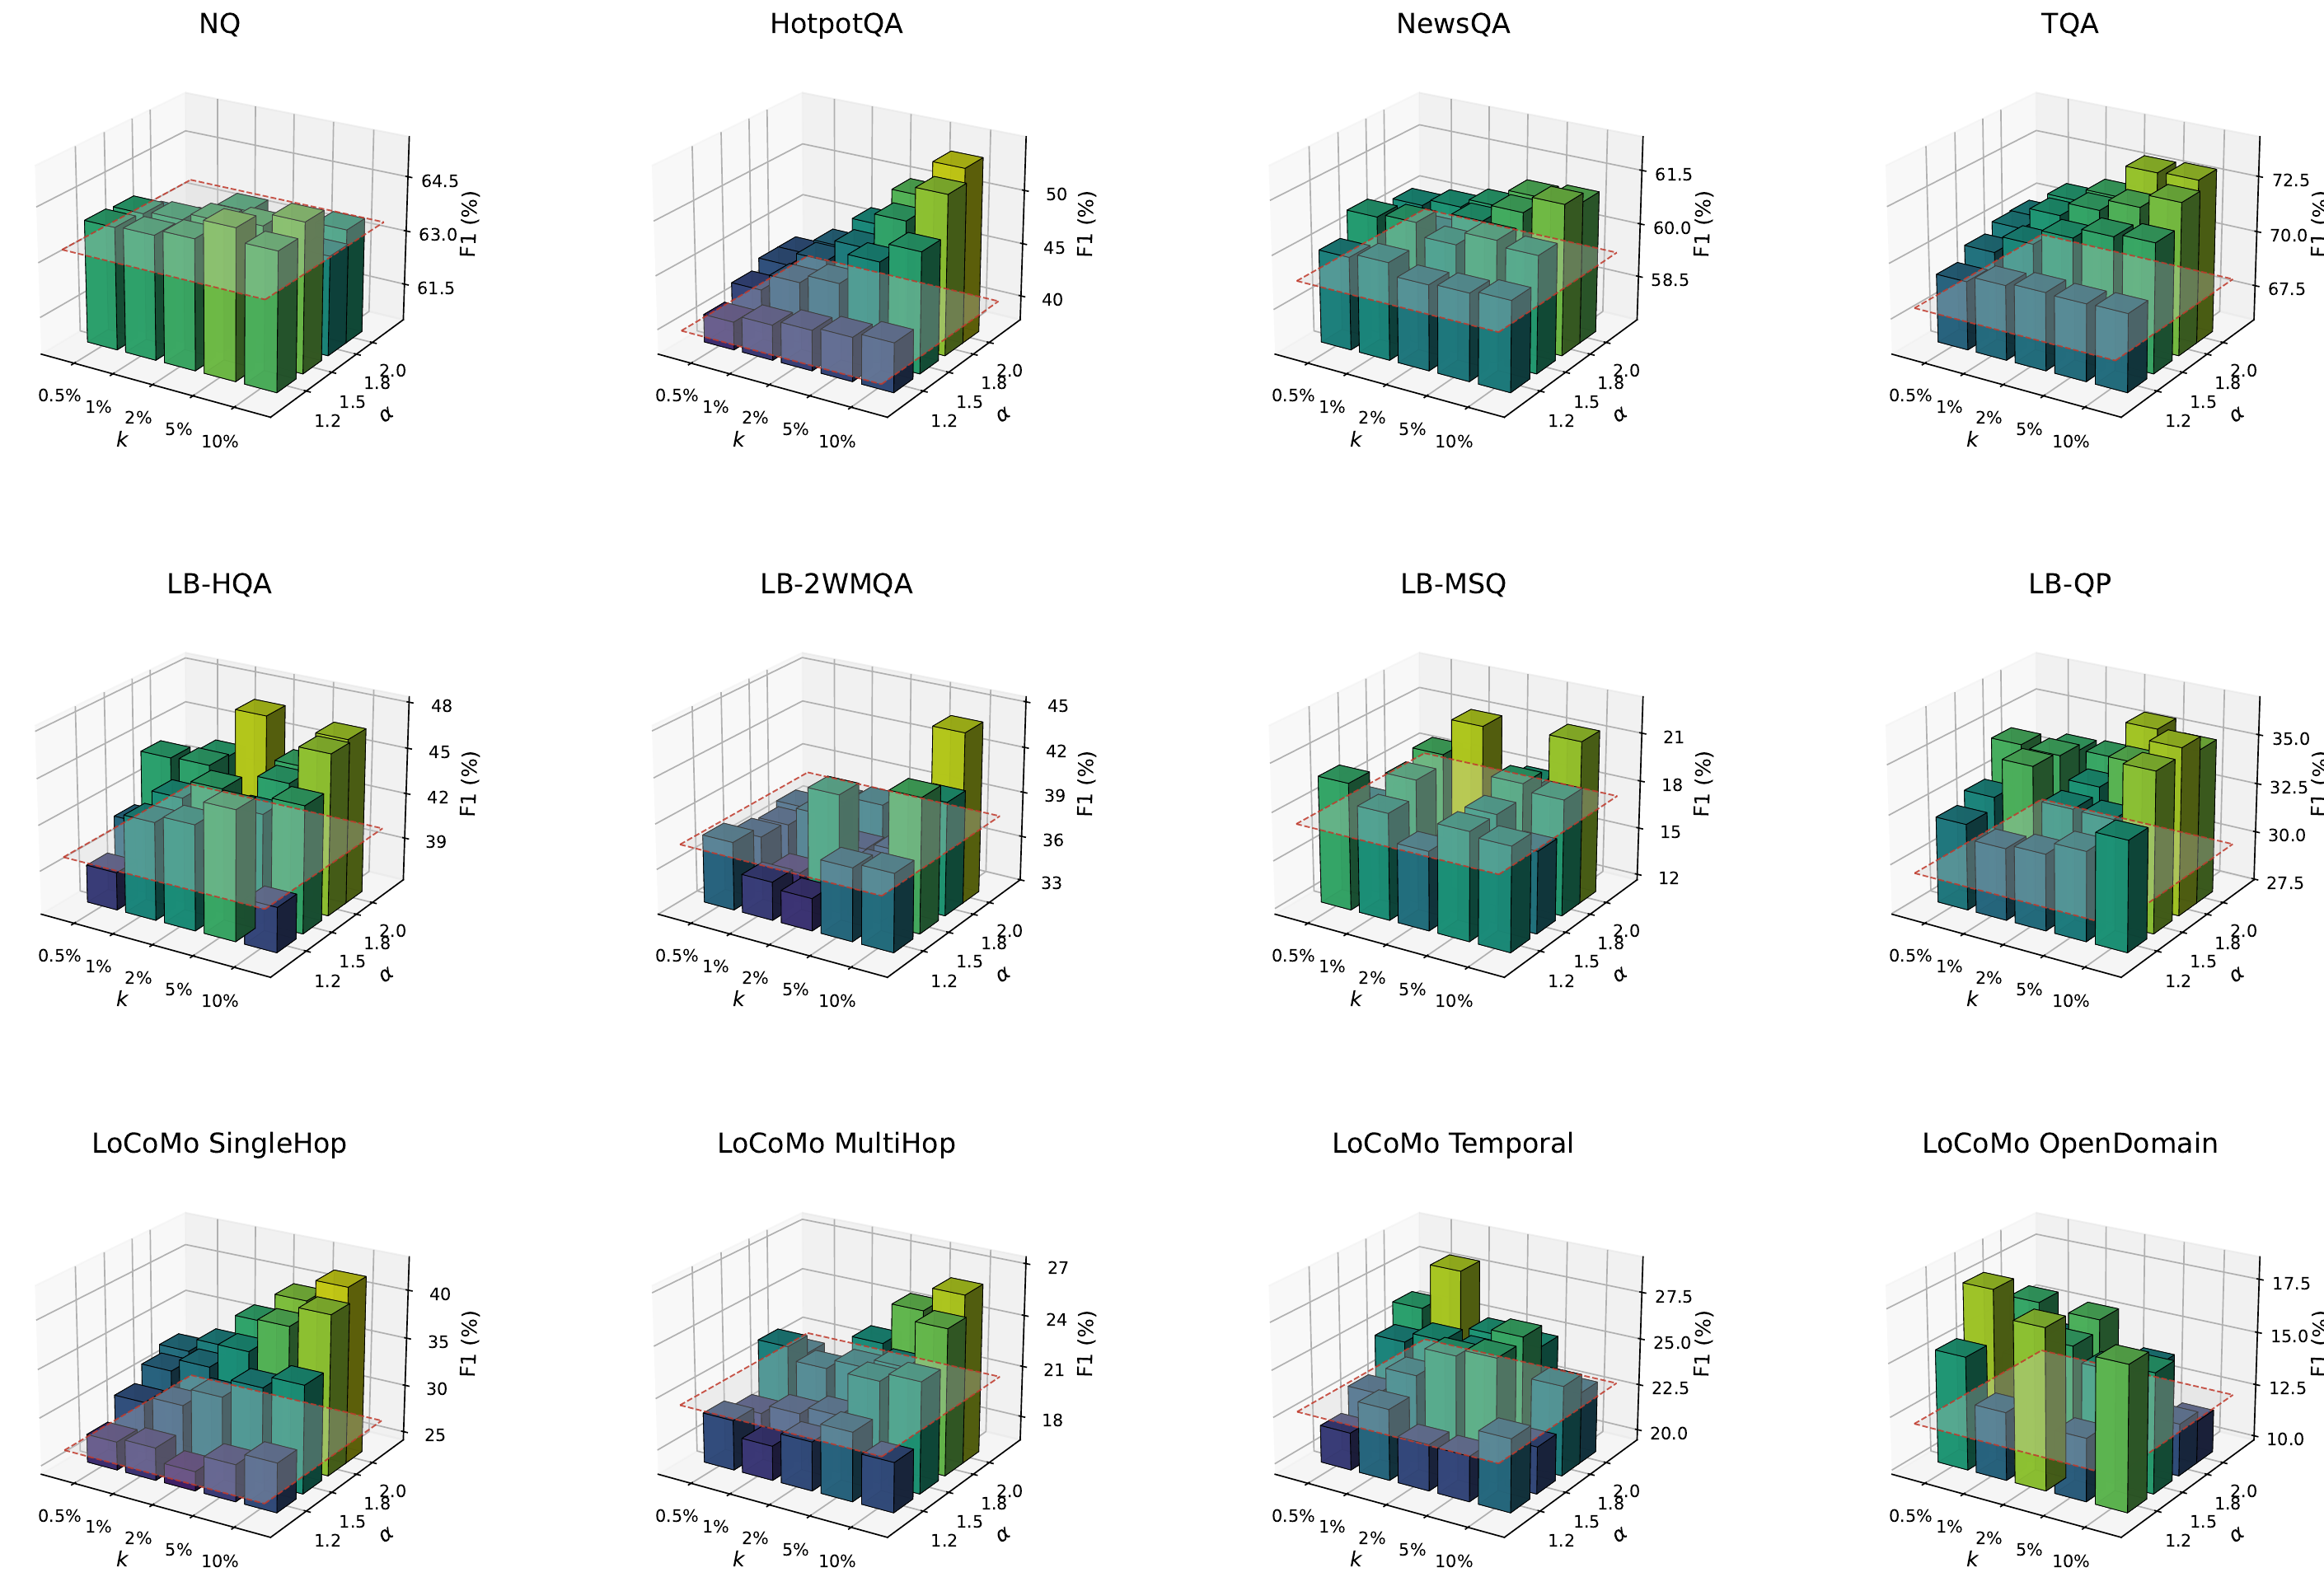}
  \caption{\textbf{Full $(k,\alpha)$ sweep on 12 datasets.} 3D bar version.
  Short-form QA (top row): NQ / HotpotQA / NewsQA / TQA. LongBench
  multi-page (middle row): LB-HQA / LB-2WMQA / LB-MSQ / LB-QP. LoCoMo
  multi-page memory (bottom row): SingleHop / MultiHop / Temporal /
  OpenDomain.}
  \label{fig:sensitivity_full}
\end{figure}

\section{Dataset Statistics}
\label{app:dataset_stats}

Table~\ref{tab:dataset_stats} summarizes the three benchmark families used in
\S\ref{sec:experiments}: short-form QA (single rendered page), LongBench
multi-page QA, and LoCoMo multi-page memory QA. Numbers are computed on the
official validation/test split of each dataset (HotpotQA in distractor mode);
context length is reported in both raw characters and whitespace-separated
words.

\begin{table}[h]
  \centering
  \footnotesize
  \setlength{\tabcolsep}{6pt}
  
  \begin{tabular}{@{}llrrr@{}}
    \toprule
    \textbf{Family} & \textbf{Dataset} & \textbf{\# Samples}
      & \textbf{Avg.\ chars} & \textbf{Avg.\ words} \\
    \midrule
    \multirow{4}{*}{\shortstack[l]{Short-form QA\\(single page)}}
      & NQ        & 12{,}836 &     843 &    159 \\
      & HotpotQA  &  7{,}404 &  5{,}479 &    897 \\
      & NewsQA    &  4{,}212 &  3{,}001 &    493 \\
      & TQA       &  7{,}785 &  4{,}064 &    673 \\
    \midrule
    \multirow{4}{*}{\shortstack[l]{LongBench\\(multi-page)}}
      & LB-HQA    &    200 &  56{,}550 &  9{,}133 \\
      & LB-2WMQA  &    200 &  29{,}615 &  4{,}873 \\
      & LB-MSQ    &    200 &  69{,}405 & 11{,}196 \\
      & LB-QP     &    200 &  23{,}641 &  3{,}599 \\
    \midrule
    Memory QA
      & LoCoMo    &  1{,}542 &  79{,}668 & 14{,}394 \\
    \bottomrule
  \end{tabular}
  \caption{Dataset statistics for the three benchmark families used in
  \S\ref{sec:experiments}. \textbf{Avg.\ chars} and \textbf{Avg.\ words}
  are the per-sample mean character and whitespace-separated word counts
  of the textual context~$T$ before rendering.}
  \label{tab:dataset_stats}
\end{table}

\section{Cross-Architecture Results}
\label{app:cross_arch}

To verify that the AGAR gain is not specific to one architecture or
post-training recipe, we additionally evaluate three other VLMs:
\textbf{InternVL3.5-8B}, \textbf{GLM-4.1V-9B-Thinking}, and
\textbf{Glyph} (a public model post-trained from GLM-4.1V-9B-Thinking
specifically for visual text comprehension). Tables~\ref{tab:cross_arch_internvl_short}--\ref{tab:cross_arch_glyph_multi}
mirror Tables~\ref{tab:exp_main_shortform}--\ref{tab:exp_main_multipage}
of the main text: one short-form and one multi-page table per model,
with the same Plain~VQA / Random / Uniform / VEA-Br / VEA-Con / AGAR
row layout. Cells we have not yet evaluated are left as ``--''.
Across the three models, AGAR delivers consistent gains over Plain
VQA on the large majority of cells (notably InternVL TQA, Glyph NewsQA
on short-form, and Glyph LoCoMo OpenDomain on multi-page are the only
material regressions); the magnitude and direction of the gain track
the same patterns observed for Qwen3-VL-8B in the main text.

% ============================================================================
% InternVL3.5-8B
% ============================================================================
\begin{table}[h]
  \centering
  \footnotesize
  \setlength{\tabcolsep}{4pt}
  
  \begin{tabular}{@{}l cccc@{}}
    \toprule
    \textbf{Method} & \textbf{NQ} & \textbf{HotpotQA} & \textbf{NewsQA} & \textbf{TQA} \\
    \midrule
    Plain VQA           & 59.1                  & 31.5                  & 44.4                  & 66.5                 \\
    Random              & --                    & --                    & --                    & --                   \\
    Uniform             & --                    & --                    & --                    & --                   \\
    VEA-Br              & 59.0\dn{0.2}          & 29.4\dn{6.7}          & 40.8\dn{8.1}          & 62.8\dn{5.6}         \\
    VEA-Con             & 59.9\up{1.4}          & 29.6\dn{6.0}          & 40.3\dn{9.2}          & 65.3\dn{1.8}         \\
    \midrule
    \textbf{AGAR (ours)}& \textbf{67.4}\up{14.0}& \textbf{32.8}\up{4.1} & \textbf{47.2}\up{6.3} & 65.9\dn{0.9}         \\
    \bottomrule
  \end{tabular}
  \caption{\textbf{InternVL3.5-8B short-form QA} (F1). Each cell shows
  F1 followed by its \emph{relative} change (\%) vs.\ Plain VQA. Plain /
  AGAR are on the full validation splits; VEA-Br / VEA-Con are on the
  $n{=}1000$ stratified subset. Random / Uniform are pending for this
  model.}
  \label{tab:cross_arch_internvl_short}
\end{table}

\begin{table}[h]
  \centering
  \footnotesize
  \setlength{\tabcolsep}{3pt}
  
  \resizebox{\linewidth}{!}{%
  \begin{tabular}{@{}l cccc | cccc@{}}
    \toprule
    & \multicolumn{4}{c|}{\textbf{LongBench (multi-page) -- F1}}
    & \multicolumn{4}{c}{\textbf{LoCoMo (multi-page memory) -- F1}} \\
    \cmidrule(lr){2-5}\cmidrule(lr){6-9}
    \textbf{Method} & \textbf{LB-HQA} & \textbf{LB-2WMQA} & \textbf{LB-MSQ} & \textbf{LB-QP}
                    & \textbf{SingleHop} & \textbf{MultiHop} & \textbf{Temporal} & \textbf{OpenDom.} \\
    \midrule
    Plain VQA           & 48.6                  & 43.1                  & 24.0                  & 37.2
                        & 35.9                  & 26.0                  & 28.1                  & 16.4                 \\
    Random              & 47.5\dn{2.3}          & 44.3\up{2.8}          & 25.5\up{6.2}          & 40.0\up{7.5}
                        & 38.6\up{7.5}          & 27.6\up{6.2}          & --                    & --                   \\
    Uniform             & 48.6\eq               & 43.1\eq               & 24.0\eq               & 37.2\eq
                        & 35.8\dn{0.3}          & --                    & --                    & 16.4\eq              \\
    VEA-Br              & --                    & 31.3\dn{27.4}         & --                    & --
                        & --                    & --                    & --                    & --                   \\
    VEA-Con             & --                    & 32.9\dn{23.7}         & --                    & --
                        & --                    & --                    & --                    & --                   \\
    \midrule
    \textbf{AGAR (ours)}& \textbf{48.9}\up{0.6} & \textbf{43.8}\up{1.6} & \textbf{25.6}\up{6.7} & \textbf{38.0}\up{2.2}
                        & \textbf{42.2}\up{17.5}& \textbf{27.6}\up{6.2} & \textbf{31.4}\up{11.7}& \textbf{17.8}\up{8.5}\\
    \bottomrule
  \end{tabular}%
  }
  \caption{\textbf{InternVL3.5-8B multi-page benchmarks} (F1). Each cell
  shows F1 followed by its \emph{relative} change (\%) vs.\ Plain VQA.
  AGAR is best on every cell. Cells without a result are still pending.}
  \label{tab:cross_arch_internvl_multi}
\end{table}

% ============================================================================
% GLM-4.1V-9B-Thinking
% ============================================================================
\begin{table}[h]
  \centering
  \footnotesize
  \setlength{\tabcolsep}{4pt}
  
  \begin{tabular}{@{}l cccc@{}}
    \toprule
    \textbf{Method} & \textbf{NQ} & \textbf{HotpotQA} & \textbf{NewsQA} & \textbf{TQA} \\
    \midrule
    Plain VQA           & 54.8                  & 40.9                  & 58.1                  & 65.1                 \\
    Random              & --                    & --                    & --                    & --                   \\
    Uniform             & --                    & --                    & --                    & --                   \\
    VEA-Br              & --                    & --                    & --                    & --                   \\
    VEA-Con             & --                    & --                    & --                    & --                   \\
    \midrule
    \textbf{AGAR (ours)}& \textbf{61.8}\up{12.8}& \textbf{48.0}\up{17.4}& \textbf{58.5}\up{0.7} & \textbf{68.1}\up{4.6}\\
    \bottomrule
  \end{tabular}
  \caption{\textbf{GLM-4.1V-9B-Thinking short-form QA} (F1). Each cell
  shows F1 followed by its \emph{relative} change (\%) vs.\ Plain VQA.
  Evaluated on the $n{=}1000$ stratified subset. Random / Uniform /
  VEA-Br / VEA-Con are pending for this model.}
  \label{tab:cross_arch_glm_short}
\end{table}

\begin{table}[h]
  \centering
  \footnotesize
  \setlength{\tabcolsep}{3pt}
  
  \resizebox{\linewidth}{!}{%
  \begin{tabular}{@{}l cccc | cccc@{}}
    \toprule
    & \multicolumn{4}{c|}{\textbf{LongBench (multi-page) -- F1}}
    & \multicolumn{4}{c}{\textbf{LoCoMo (multi-page memory) -- F1}} \\
    \cmidrule(lr){2-5}\cmidrule(lr){6-9}
    \textbf{Method} & \textbf{LB-HQA} & \textbf{LB-2WMQA} & \textbf{LB-MSQ} & \textbf{LB-QP}
                    & \textbf{SingleHop} & \textbf{MultiHop} & \textbf{Temporal} & \textbf{OpenDom.} \\
    \midrule
    Plain VQA           & 44.5                  & 50.1                  & 24.8                  & 24.8
                        & 29.2                  & 17.8                  & 11.9                  & 13.7                 \\
    Random              & --                    & 46.5\dn{7.2}          & --                    & --
                        & --                    & --                    & 11.5\dn{3.4}          & --                   \\
    Uniform             & 44.5\eq               & 50.9\up{1.6}          & --                    & --
                        & --                    & 17.8\eq               & --                    & --                   \\
    VEA-Br              & 46.7\up{4.9}          & --                    & --                    & --
                        & --                    & 17.8\eq               & --                    & --                   \\
    VEA-Con             & 45.9\up{3.1}          & --                    & --                    & --
                        & --                    & 18.3\up{2.8}          & --                    & --                   \\
    \midrule
    \textbf{AGAR (ours)}& \textbf{46.9}\up{5.4} & \textbf{50.7}\up{1.2} & \textbf{26.8}\up{8.1} & 24.8\eq
                        & \textbf{32.7}\up{12.0}& \textbf{22.0}\up{23.6}& \textbf{13.5}\up{13.4}& \textbf{16.2}\up{18.2}\\
    \bottomrule
  \end{tabular}%
  }
  \caption{\textbf{GLM-4.1V-9B-Thinking multi-page benchmarks} (F1).
  Each cell shows F1 followed by its \emph{relative} change (\%) vs.\
  Plain VQA. AGAR is best on every fully-populated row; baseline
  coverage is partial.}
  \label{tab:cross_arch_glm_multi}
\end{table}

% ============================================================================
% Glyph
% ============================================================================
\begin{table}[h]
  \centering
  \footnotesize
  \setlength{\tabcolsep}{4pt}
  
  \begin{tabular}{@{}l cccc@{}}
    \toprule
    \textbf{Method} & \textbf{NQ} & \textbf{HotpotQA} & \textbf{NewsQA} & \textbf{TQA} \\
    \midrule
    Plain VQA           & 59.3                  & 56.4                  & 57.1                  & 75.8                 \\
    Random              & --                    & --                    & --                    & --                   \\
    Uniform             & --                    & --                    & --                    & --                   \\
    VEA-Br              & --                    & --                    & --                    & --                   \\
    VEA-Con             & --                    & --                    & --                    & --                   \\
    \midrule
    \textbf{AGAR (ours)}& \textbf{67.8}\up{14.3}& \textbf{59.6}\up{5.7} & 56.6\dn{0.9}          & \textbf{77.3}\up{2.0}\\
    \bottomrule
  \end{tabular}
  \caption{\textbf{Glyph short-form QA} (F1). Each cell shows F1
  followed by its \emph{relative} change (\%) vs.\ Plain VQA. Evaluated
  on the $n{=}1000$ stratified subset. Random / Uniform / VEA-Br /
  VEA-Con are pending.}
  \label{tab:cross_arch_glyph_short}
\end{table}

\begin{table}[h]
  \centering
  \footnotesize
  \setlength{\tabcolsep}{3pt}
  
  \resizebox{\linewidth}{!}{%
  \begin{tabular}{@{}l cccc | cccc@{}}
    \toprule
    & \multicolumn{4}{c|}{\textbf{LongBench (multi-page) -- F1}}
    & \multicolumn{4}{c}{\textbf{LoCoMo (multi-page memory) -- F1}} \\
    \cmidrule(lr){2-5}\cmidrule(lr){6-9}
    \textbf{Method} & \textbf{LB-HQA} & \textbf{LB-2WMQA} & \textbf{LB-MSQ} & \textbf{LB-QP}
                    & \textbf{SingleHop} & \textbf{MultiHop} & \textbf{Temporal} & \textbf{OpenDom.} \\
    \midrule
    Plain VQA           & 61.9                  & 68.2                  & 45.7                  & 38.4
                        & 42.0                  & 29.1                  & 21.2                  & 23.0                 \\
    Random              & --                    & --                    & --                    & --
                        & --                    & --                    & --                    & --                   \\
    Uniform             & --                    & --                    & --                    & --
                        & --                    & --                    & --                    & --                   \\
    VEA-Br              & --                    & --                    & --                    & --
                        & --                    & --                    & --                    & --                   \\
    VEA-Con             & --                    & --                    & --                    & --
                        & --                    & --                    & --                    & --                   \\
    \midrule
    \textbf{AGAR (ours)}& \textbf{62.6}\up{1.1} & \textbf{71.5}\up{4.8} & \textbf{51.2}\up{12.0}& \textbf{39.4}\up{2.6}
                        & \textbf{43.5}\up{3.6} & \textbf{29.7}\up{2.1} & \textbf{22.2}\up{4.7} & 14.6\dn{36.5}        \\
    \bottomrule
  \end{tabular}%
  }
  \caption{\textbf{Glyph multi-page benchmarks} (F1). Each cell shows
  F1 followed by its \emph{relative} change (\%) vs.\ Plain VQA. AGAR
  improves on 7/8 cells; LoCoMo OpenDomain regresses ($-36.5\%$),
  consistent with the per-sample pattern flagged for Glyph. Random /
  Uniform / VEA-Br / VEA-Con are pending.}
  \label{tab:cross_arch_glyph_multi}
\end{table}

\section{Baseline implementation}

\paragraph{\CGR.}
\CGR{}~\cite{} operates in two stages. First, the model is prompted with the rendered image and question to extract relevant content as structured textual evidence (verbatim snippets, names, dates, numbers, and brief surrounding context). Second, this extracted text is concatenated with the original question and passed to a text-only stage that produces the final answer, abstaining when evidence is insufficient.
\paragraph{\VAR.}
\VAR{}~\cite{} constructs a binary visual mask from the model's final-layer attention scores. We aggregate attention across heads, select the globally highest-scoring patches, and present the model with a version of the image in which those patches are highlighted and the remainder is unchanged.
\paragraph{\AGLA.}
\AGLA{}~\cite{} is run using the official codebase and default hyperparameters. The method produces a question-conditioned saliency map, masks out low-relevance regions to form a local-evidence image, and ensembles generations from the original and masked images via AGLA decoding. No AGLA-specific parameters were tuned on our evaluation sets.

\section{Token-Base Size Ablation}
\providecommand{\PlainVQA}{\textsc{PlainVQA}}
\providecommand{\TokenBase}{\textsc{TokenBase}}
\providecommand{\FixedTB}{\textsc{TokenBase-Fixed}}
\providecommand{\RelativeTB}{\textsc{TokenBase-Relative}}

This section provides a detailed breakdown of the compressed-regime results
in Figures~\ref{fig:qwen-tokenbase-fixed} and~\ref{fig:qwen-tokenbase-relative}.
We evaluate Qwen3-VL-8B-Instruct on HotpotQA ($n{=}1000$) and LB-QP ($n{=}200$)
at two compression levels where legibility is most degraded: 5$\times$ with a
5\,px base font, and 10$\times$ with a 3\,px base font.  In all conditions,
\TokenBase{} selects the top 2\% of attention patches and enhances them under
one of two rules:

\begin{itemize}
    \item \FixedTB{} restores selected regions to 13.5\,px regardless of the
    compressed base font.
    \item \RelativeTB{} scales selected regions by $1.5{\times}$, yielding
    7.5\,px at 5$\times$ and 4.5\,px at 10$\times$ compression.
\end{itemize}

\begin{figure}[t]
\centering
\includegraphics[width=\linewidth]{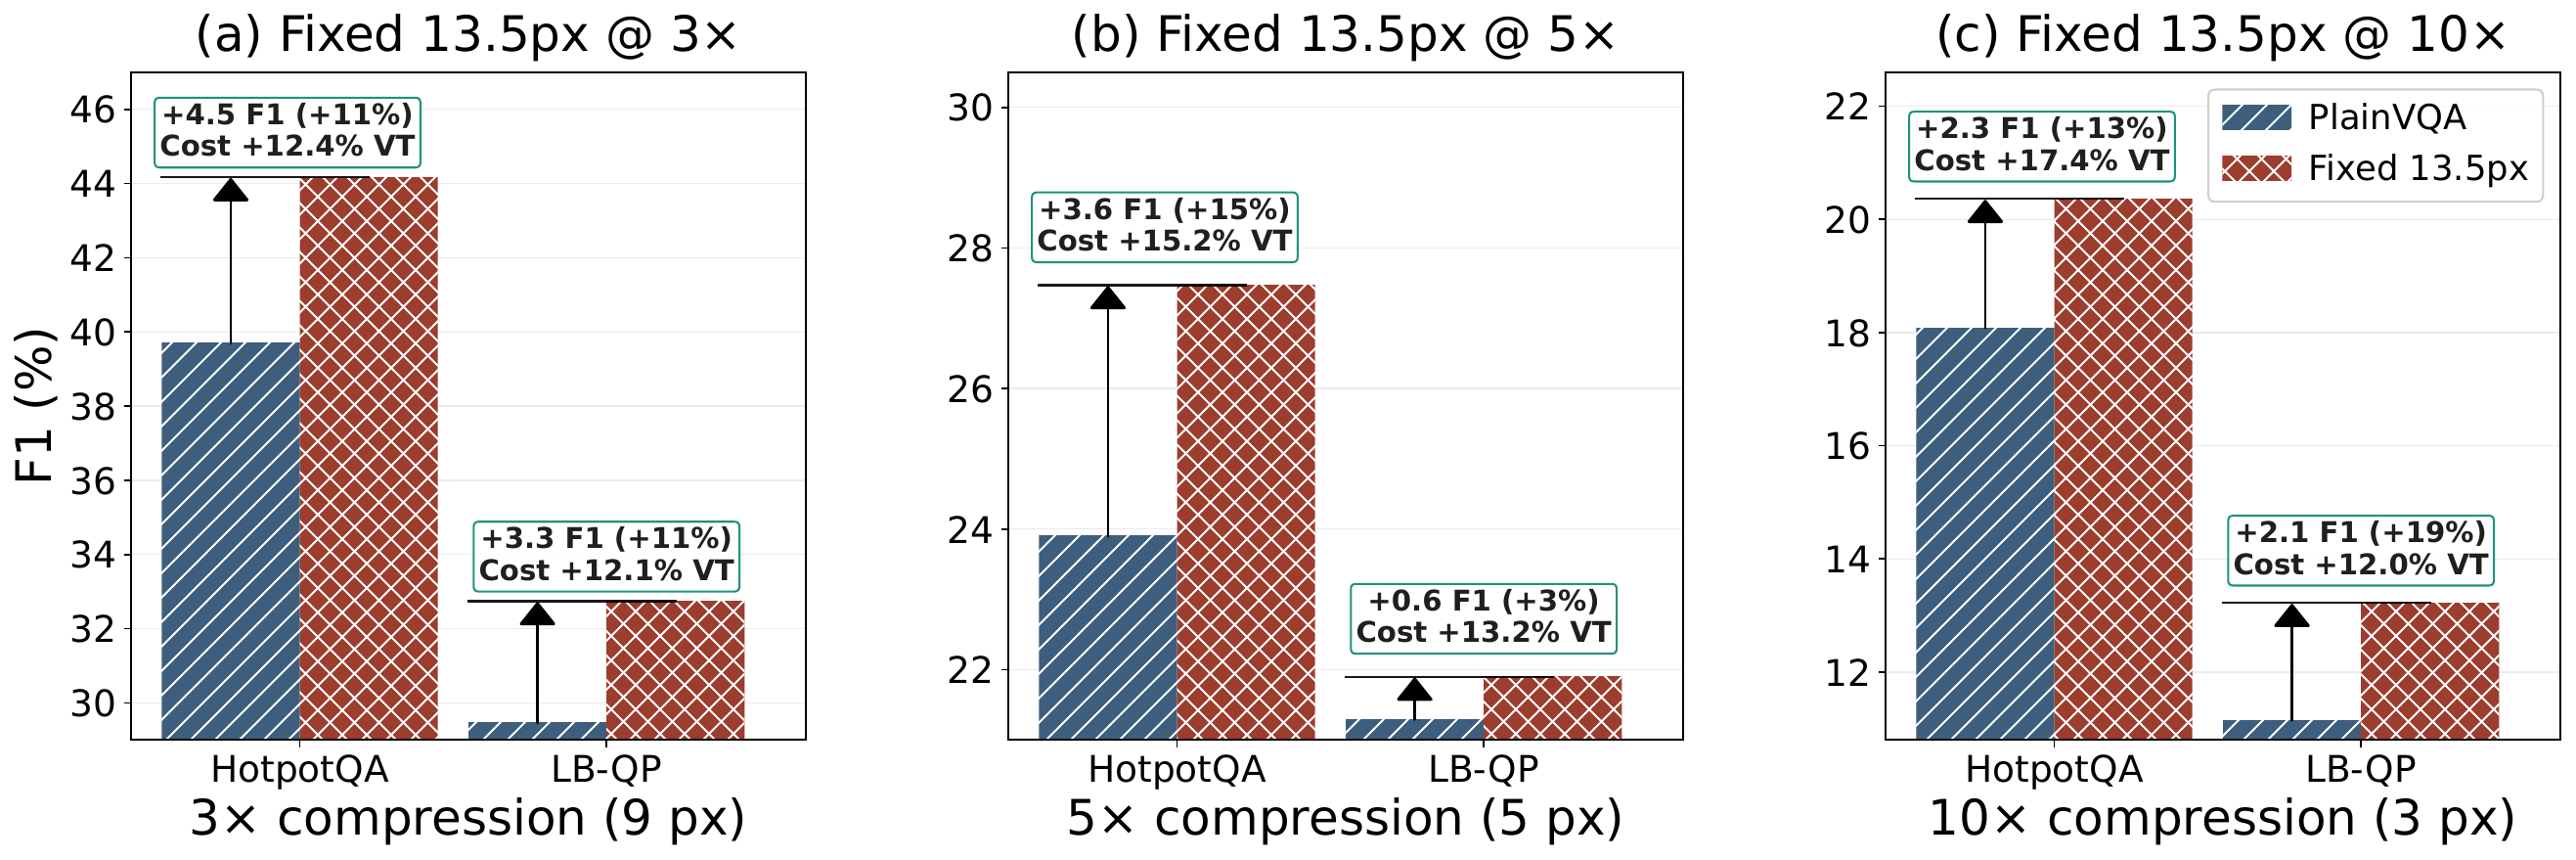}
\caption{\textbf{Fixed readable-size \TokenBase{} under
vision-token compression.} Blue: \PlainVQA{} F1; red: \FixedTB{} F1; box:
absolute and relative $\Delta$F1 plus vision-token cost (VT).  Panel (a) averages
HotpotQA and LB-QP; panels (b) and (c) show dataset-level results at 5x / 5 px
and 10x / 3 px.}
\label{fig:qwen-tokenbase-fixed}
\end{figure}

\begin{figure}[t]
\centering
\includegraphics[width=\linewidth]{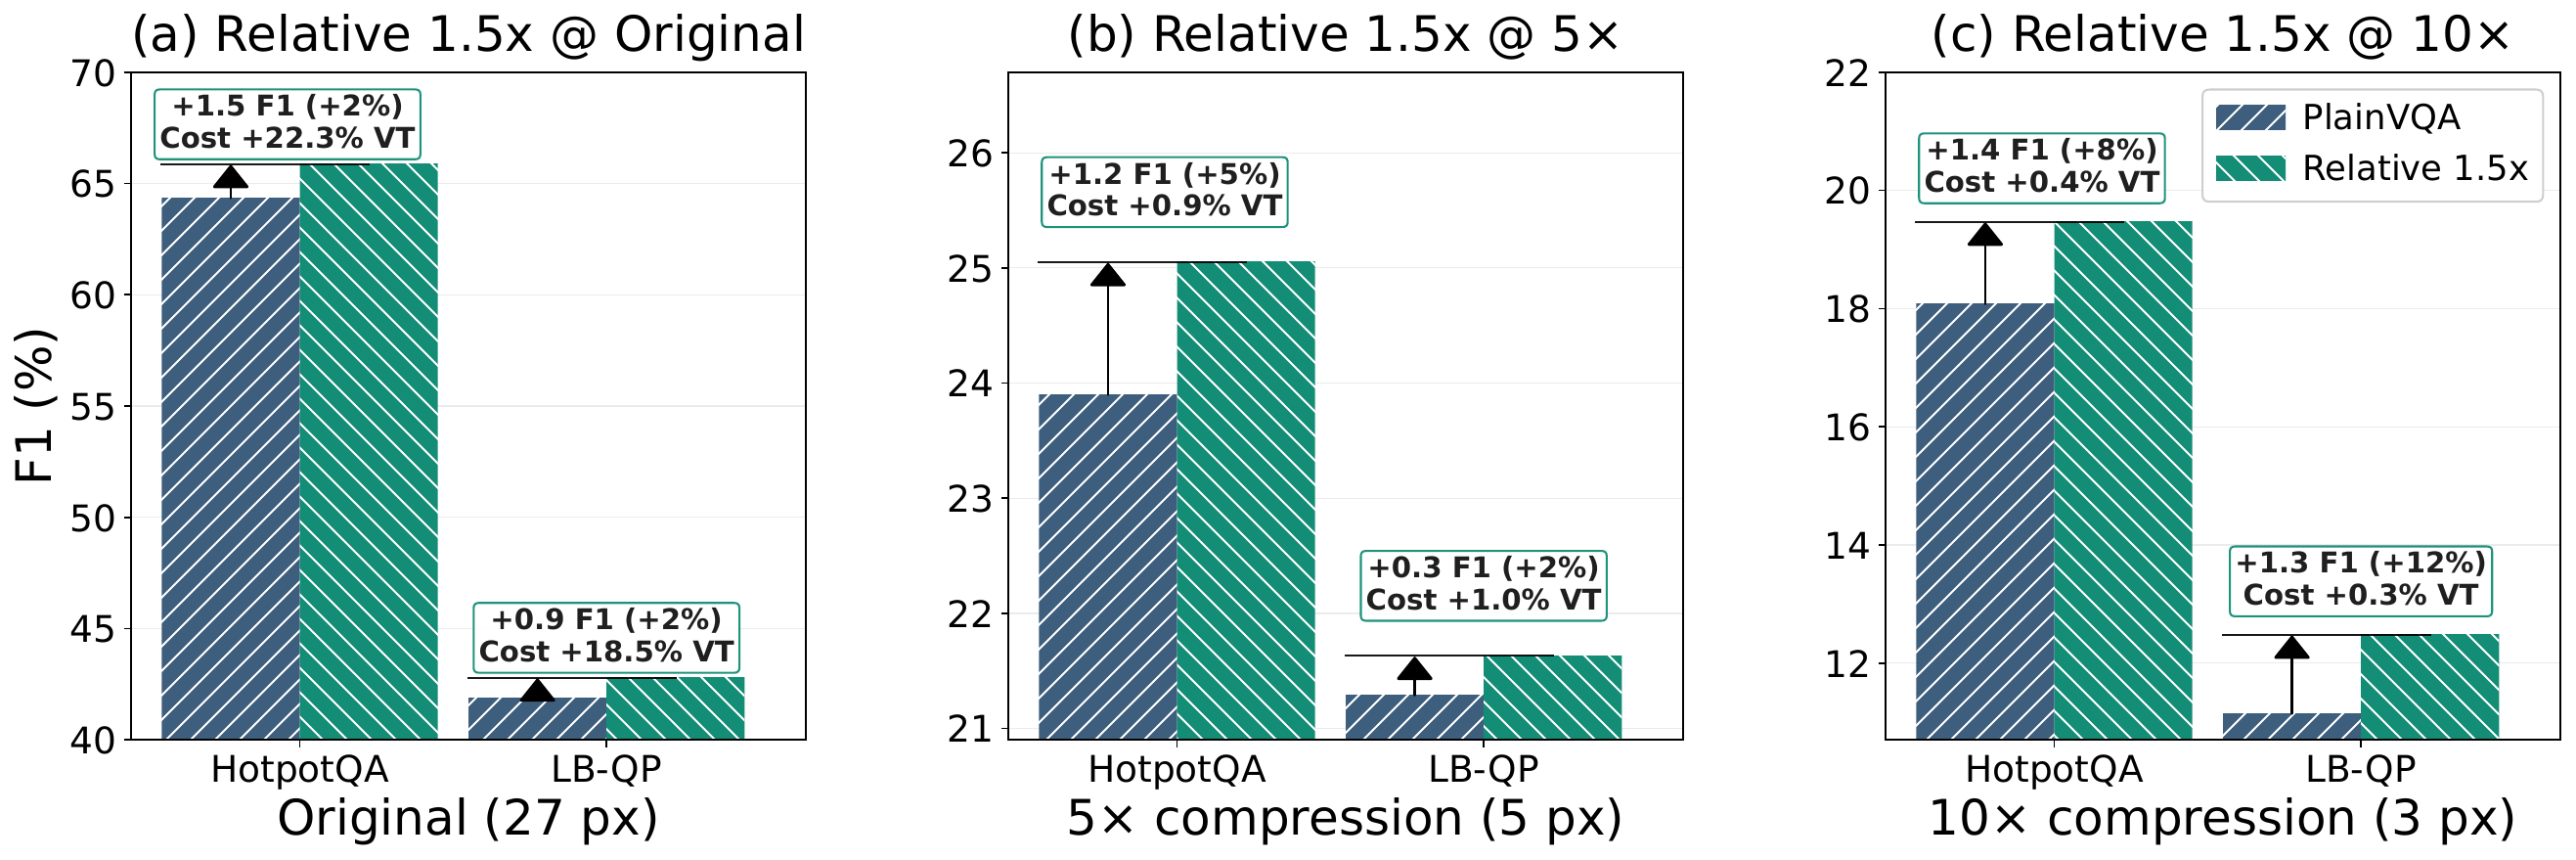}
\caption{\textbf{Relative \TokenBase{} under vision-token
compression.} Blue: \PlainVQA{} F1; green: \RelativeTB{} F1; box: absolute and
relative $\Delta$F1 plus vision-token cost (VT).  Panel (a) averages HotpotQA and
LB-QP; panels (b) and (c) show dataset-level results at 5x / 5 px and 10x /
3 px.}
\label{fig:qwen-tokenbase-relative}
\end{figure}

\paragraph{Main observation.}
Under strong compression, fixed readable-size restoration gives the better
accuracy--cost trade-off among the two enhancement rules.  Averaged over
HotpotQA and LB-QP, \FixedTB{} gains +2.1 F1 at 5x and +2.2 F1 at 10x, while
\RelativeTB{} gains +0.7 F1 and +1.4 F1.  The conclusion is not merely that
``more vision tokens help'': if this were the whole story, reporting only F1
would be misleading.  We therefore report the vision-token cost next to every
F1 gain.  The cost of \FixedTB{} is real, about +14--15\% average vision tokens
relative to compressed \PlainVQA{}.  \RelativeTB{} is much cheaper, adding only
+0.9\% at 5x and +0.3\% at 10x on average, but it also recovers less F1.  The
extra budget used by \FixedTB{} is targeted to selected evidence regions rather
than spent by globally increasing the entire page rendering.

\paragraph{Why relative enlargement is weaker.}
\RelativeTB{} gives a useful sanity check: it changes the selected regions
while barely changing the token budget.  The result is positive but smaller
than \FixedTB{}, which suggests that the bottleneck is not simply selecting the
right patches.  Under 5 px and 3 px rendering, the selected evidence also needs
to cross an absolute readability threshold.  A $1.5{\times}$ relative scale
leaves the selected text at 7.5 px or 4.5 px; fixed restoration moves the same
selected regions to 13.5 px.  Our finding is therefore that compressed
document QA needs a readable lower bound for attended evidence, not only a
relative zoom.

\paragraph{Takeaway.}
The two figures motivate a conditional design rule for compressed visual QA:
relative enlargement is attractive when budget overhead must be minimal, but it
does not fully solve the readability failure caused by 5 px and 3 px text.
Fixed readable-size restoration spends a clearly reported amount of extra
vision-token budget and produces consistently larger F1 gains on the plotted
compressed Qwen settings.  For compressed documents, the relevant design target
is therefore not a single global scale factor, but a readable lower bound for
the selected evidence regions.

\section{Case study}
\begin{figure}[h]
  \centering
  \includegraphics[width=\linewidth]{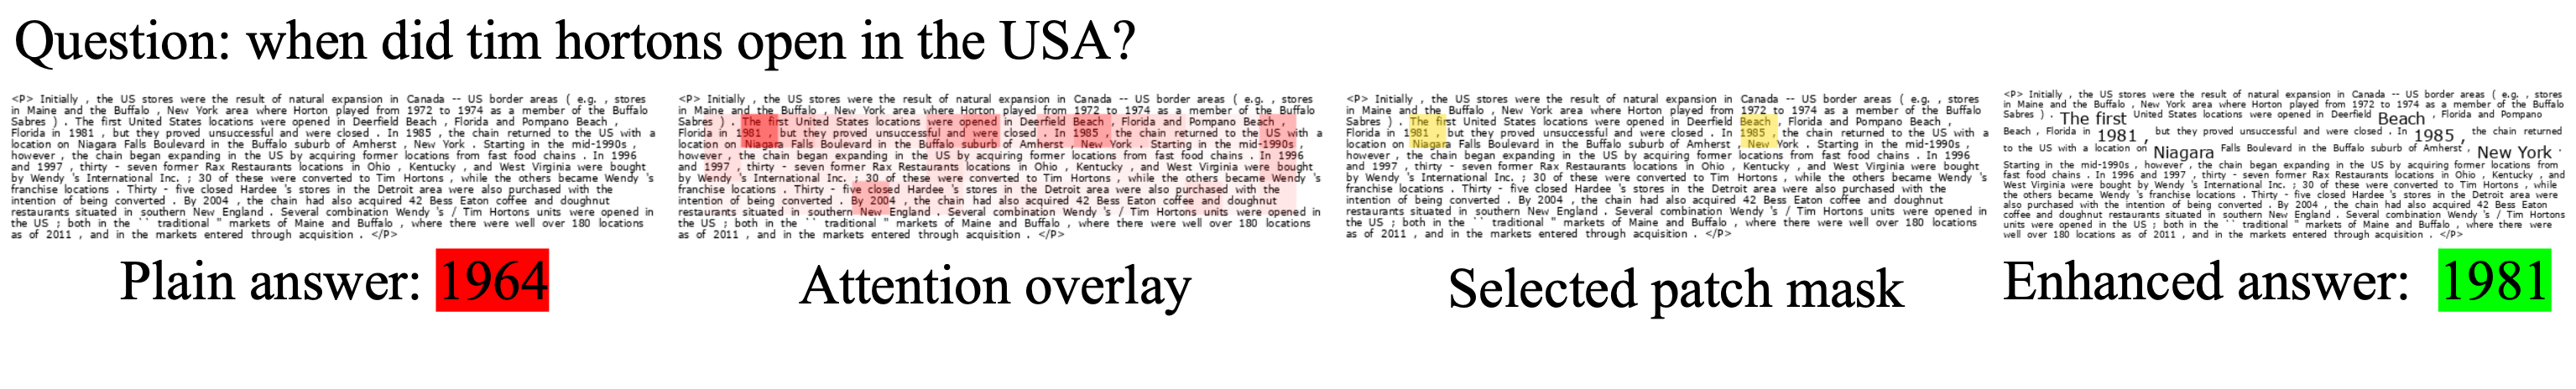}
  \caption{}
  \label{fig:locomo_1singlehop}
\end{figure}

\begin{figure}[h]
  \centering
  \includegraphics[width=\linewidth]{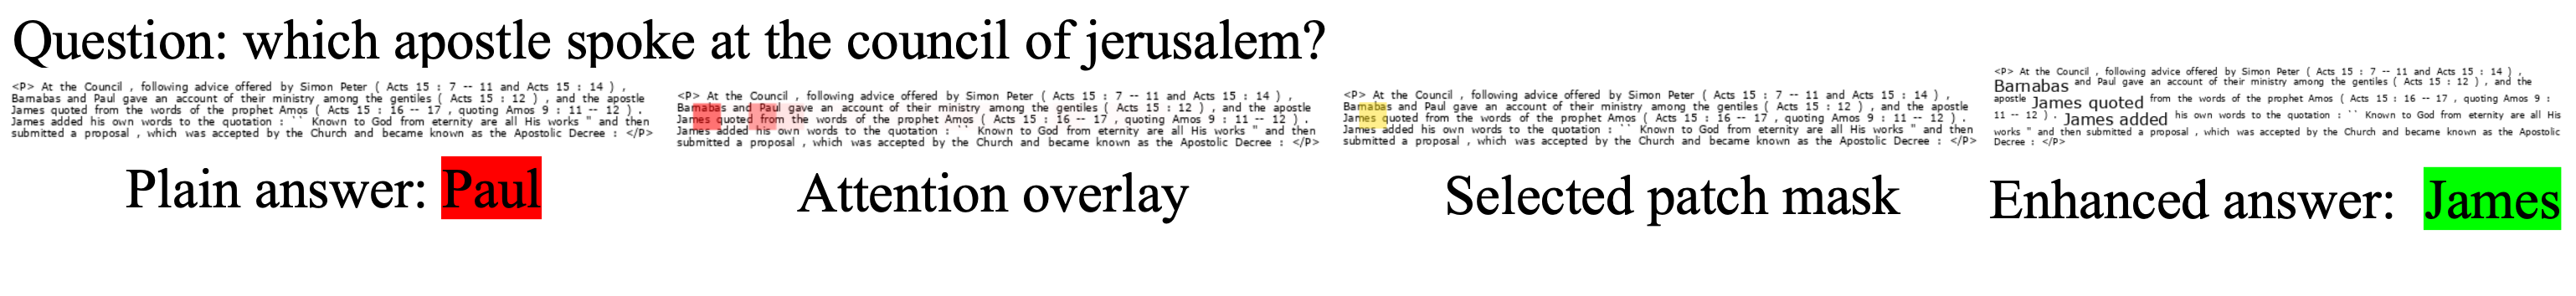}
  \caption{}
  \label{fig:locomo_1singlehop}
\end{figure}

\begin{figure}[h]
  \centering
  \includegraphics[width=\linewidth]{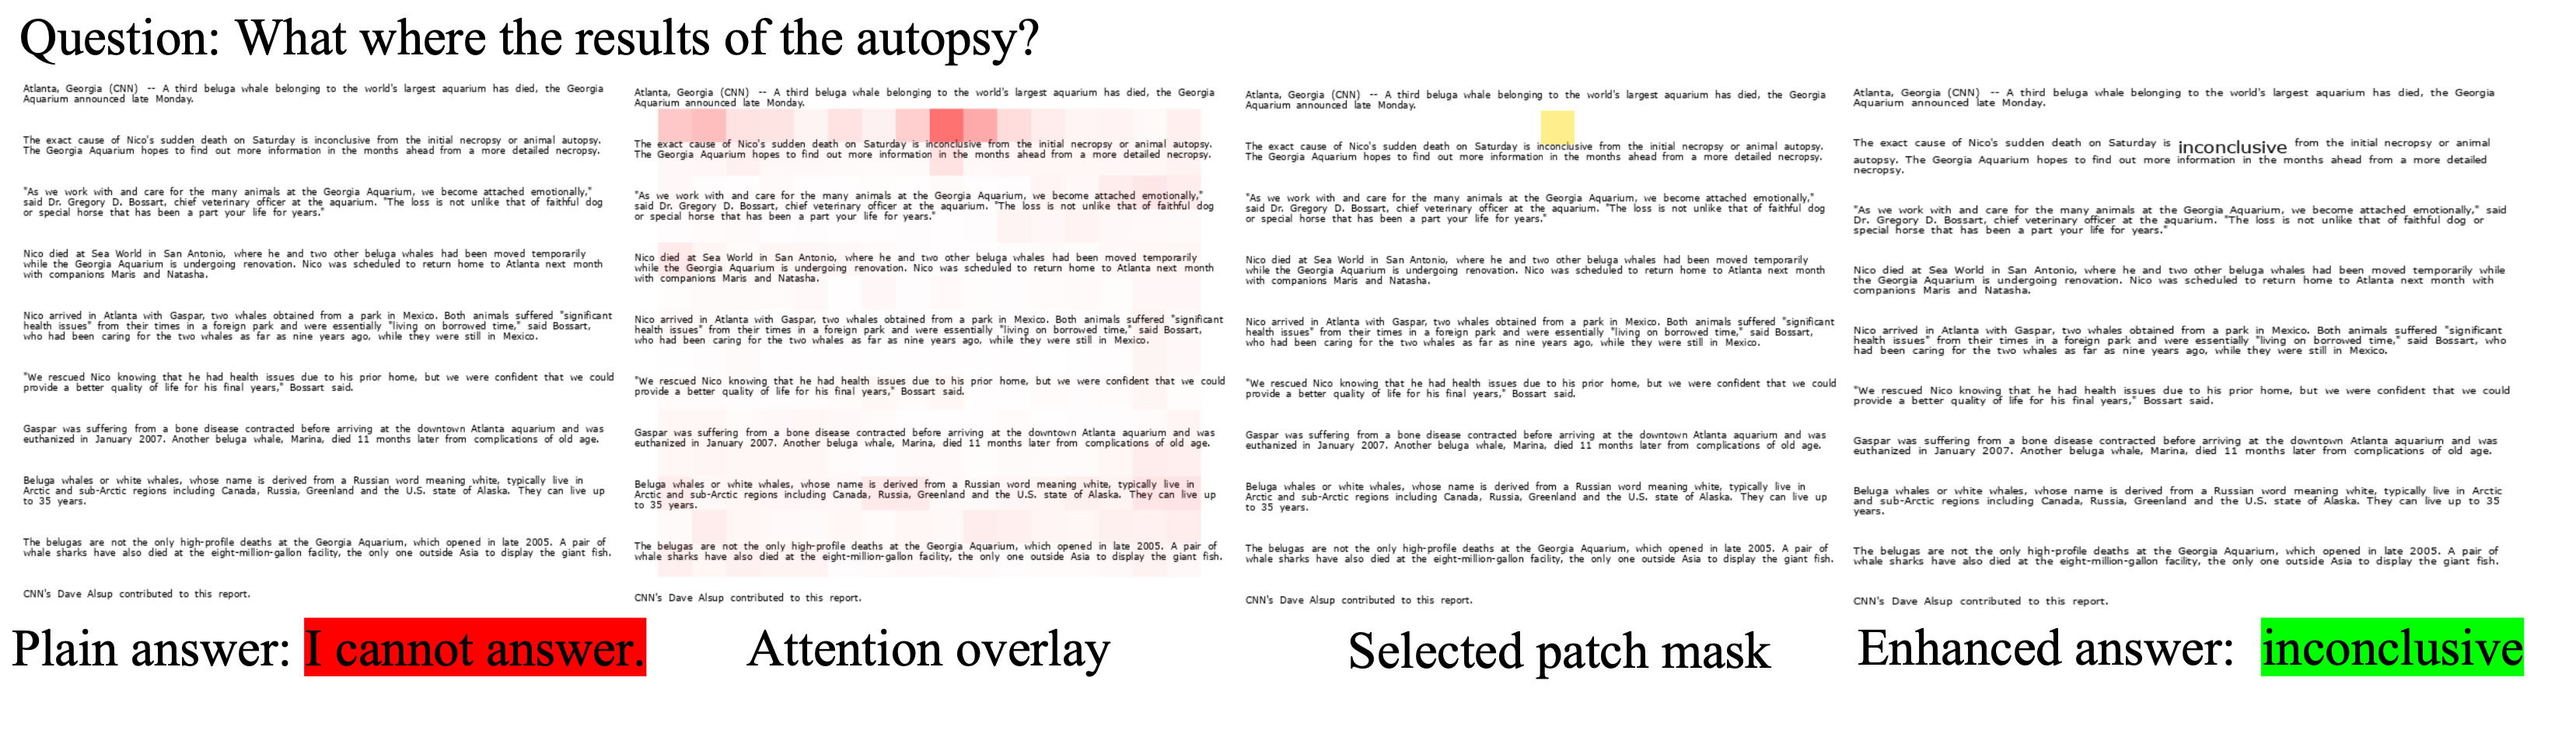}
  \caption{}
  \label{fig:locomo_1singlehop}
\end{figure}

\begin{figure}[h]
  \centering
  \includegraphics[width=\linewidth]{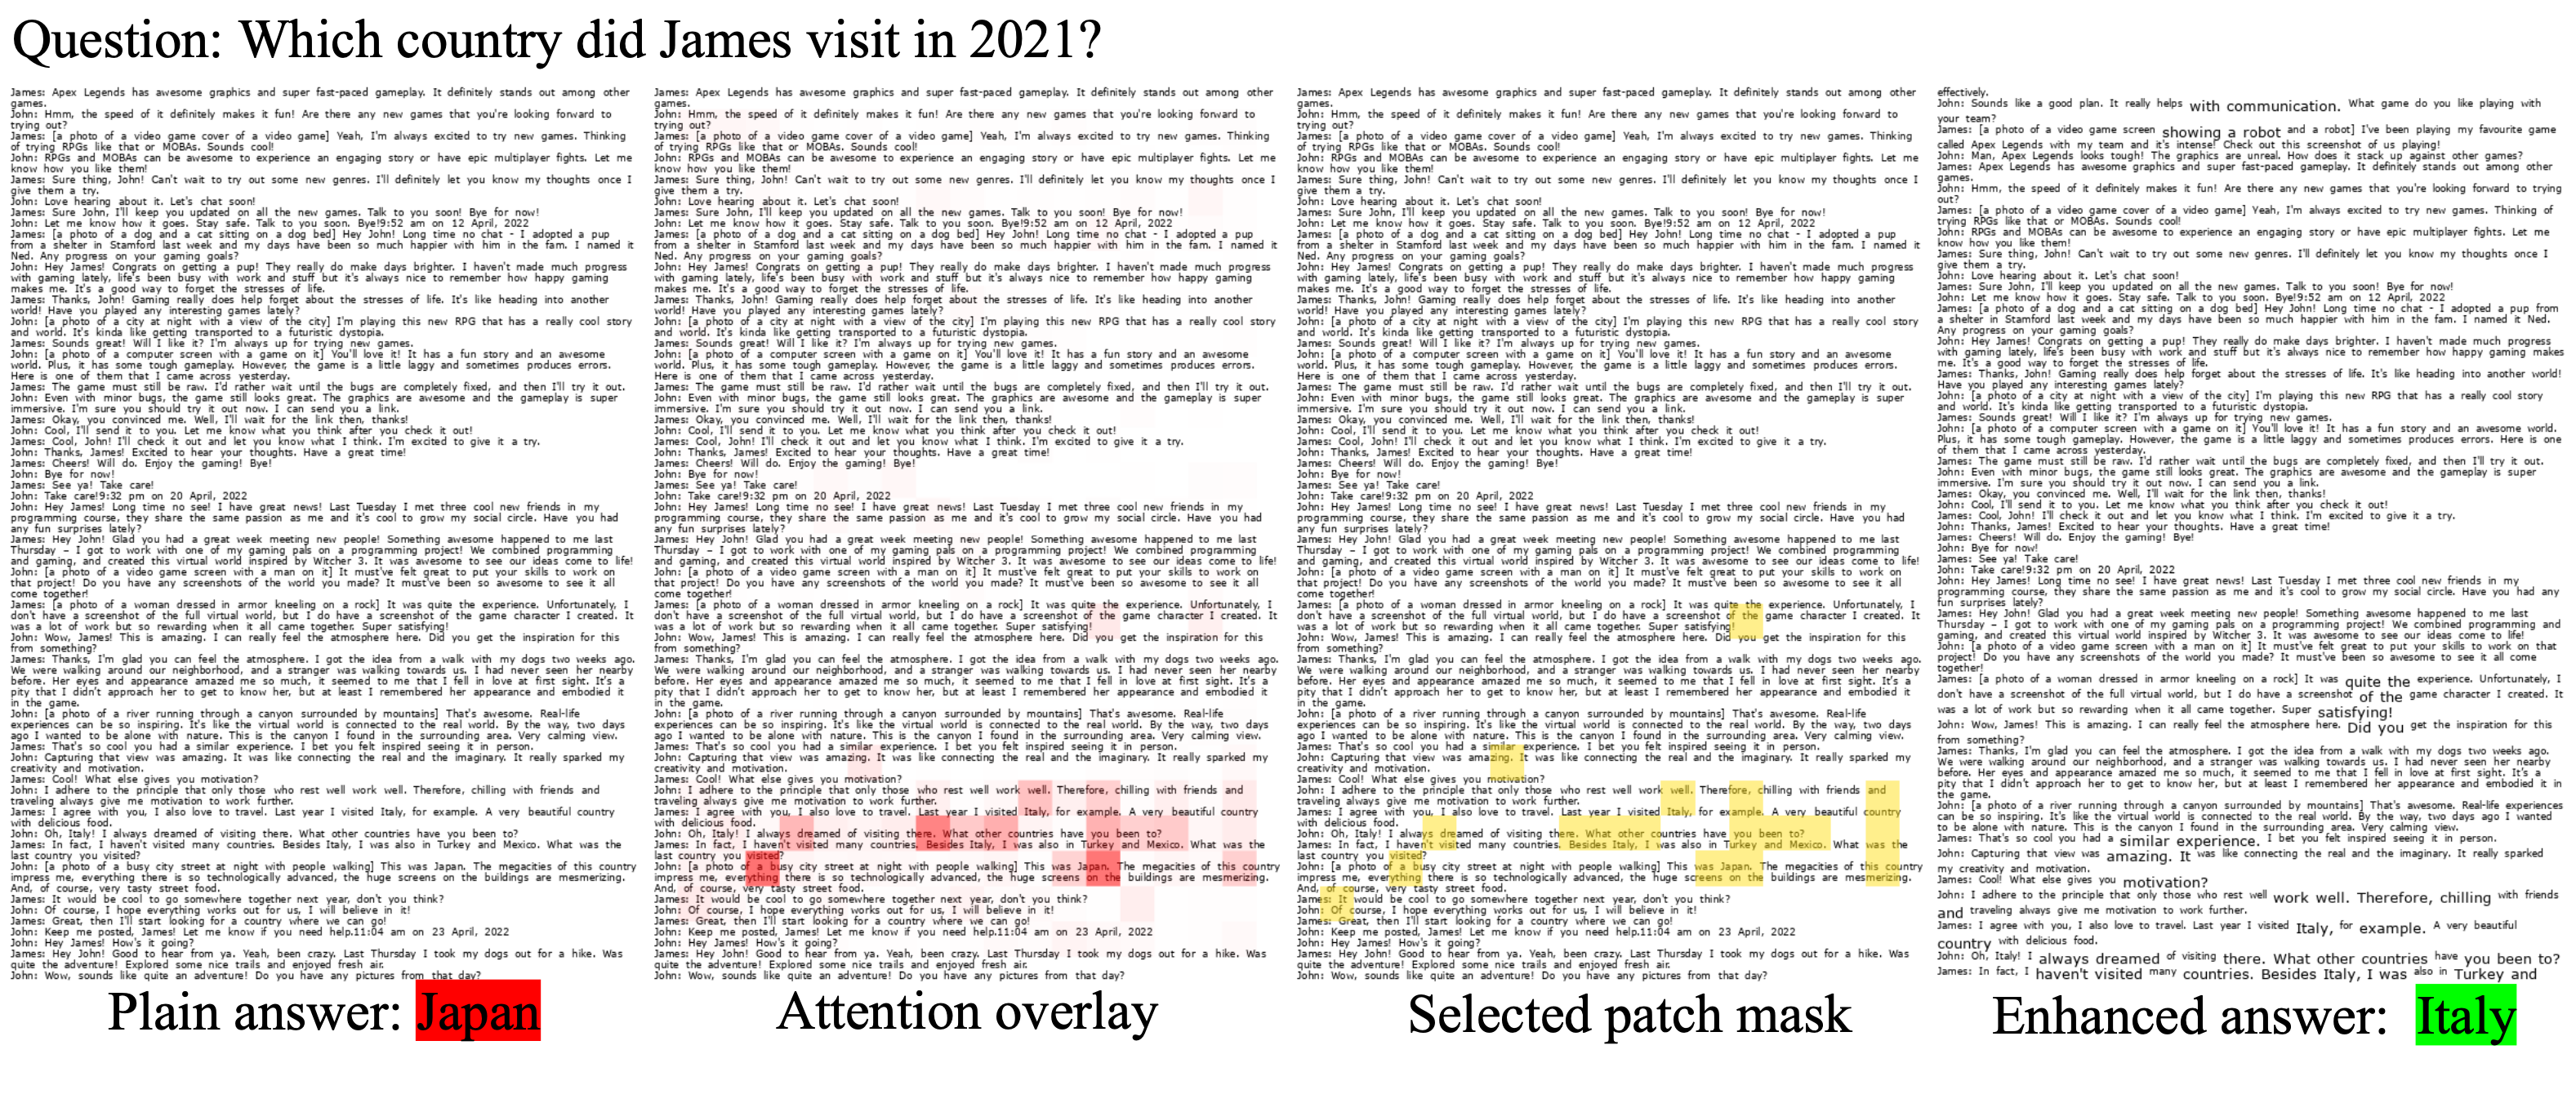}
  \caption{}
  \label{fig:locomo_1singlehop}
\end{figure}
